# Supplementary material for: From the generalized reflection law to the realization of perfect anomalous reflectors
Source: arXiv:1609.08041 source file (2017-04-13)
Supplement: Supplementary file 1 [file Supplemantary_material.pdf]

Supplementary material for the paper

# "From the generalized reflection law to the realization of perfect anomalous reflectors"

A. Díaz-Rubio, V. S. Asadchy, A. Elsakka, and S. A. Tretyakov

## 1 Power modulation produced by reflective metasurfaces

Considering TE-polarization (electric field polarized in $y$-direction), see Fig. 1 in the main text, electric and magnetic vectors can be decomposed in the tangential and longitudinal components as:

$$\mathbf{E}(x,z) = E_t(x,z)\,\hat{y}, \tag{1}$$

$$\mathbf{H}(x,z) = H_t(x,z)\,\hat{y} + H_z(x,z)\,\hat{z}. \tag{2}$$

The metasurface is located in the $xy$-plane and it is illuminated by a plane wave with amplitude $E_\mathrm{i}$ and direction $\theta_\mathrm{i}$. The incident energy is reflected into another plane wave with amplitude $E_\mathrm{r}$ and direction $\theta_\mathrm{r}$. In this scenario, the electric and magnetic field components can be written as:

$$E_\mathrm{t}(x,z) = E_\mathrm{i} e^{-jk_1\sin\theta_\mathrm{i}x} e^{jk_1\cos\theta_\mathrm{i}z} + E_\mathrm{r} e^{-jk_1\sin\theta_\mathrm{r}x} e^{-jk_1\cos\theta_\mathrm{r}z}, \tag{3}$$

$$H_\mathrm{t}(x,z) = \frac{1}{\eta_1}\left(E_\mathrm{i}\cos\theta_\mathrm{i} e^{-jk_1\sin\theta_\mathrm{i}x} e^{jk_1\cos\theta_\mathrm{i}z} - E_\mathrm{r}\cos\theta_\mathrm{r} e^{-jk_1\sin\theta_\mathrm{r}x} e^{-jk_1\cos\theta_\mathrm{r}z}\right), \tag{4}$$

$$H_z(x,z) = \frac{1}{\eta_1}\left(E_\mathrm{i}\sin\theta_\mathrm{i} e^{-jk_1\sin\theta_\mathrm{i}x} e^{jk_1\cos\theta_\mathrm{i}z} + E_\mathrm{r}\sin\theta_\mathrm{r} e^{-jk_1\sin\theta_\mathrm{r}x} e^{-jk_1\cos\theta_\mathrm{r}z}\right). \tag{5}$$

Here, the time-harmonic dependence in the form $e^{j\omega t}$ is assumed. The Poynting vector can be expressed as:

$$P(x,z) = \frac{1}{2}\mathrm{Re}\{E_\mathrm{t}(x,z)H_\mathrm{z}(x,z)^*\}\hat{x} - \frac{1}{2}\mathrm{Re}\{E_\mathrm{t}(x,z)H_\mathrm{t}(x,z)^*\}\hat{z}. \tag{6}$$

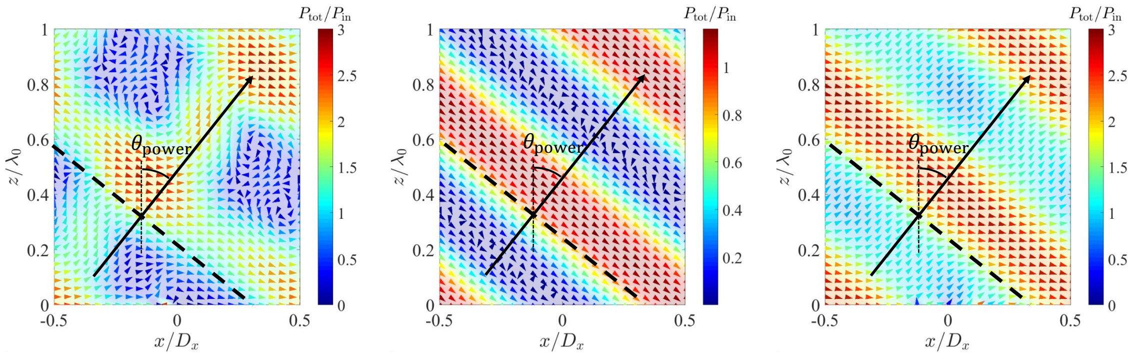


Figure 1: Total power density distribution for the conventional, lossy and active designs (from left to right.)

The Poynting vector is represented in Fig. 1 for the conventional, lossy, and active designs (from left to right). These results show that the amplitude of the power flow is modulated in the $xz$-plane with a flat wavefront. The magnitude of the power flow vector can be found as $|P(x,z)| = \sqrt{P_x(x,z)^2 + P_z(x,z)^2}$, with $P_x(x,z)$ and $P_z(x,z)$ being the $x$-component and the $z$-component of the Poynting vector. The angle of the modulation can be easily found as

$$\sin\theta_\mathrm{power} = \frac{\partial|P(x,z)|/\partial x}{\partial|P(x,z)|/\partial z} = \frac{\sin\theta_\mathrm{r} - \sin\theta_\mathrm{i}}{\cos\theta_\mathrm{r} + \cos\theta_\mathrm{i}}. \tag{7}$$

It is important to notice that the angle of the modulation is not affected by the amplitude of the reflected wave, as it is shown in Fig. 1, where lossy and active designs have the

same modulation angle. Also we can see that the power modulation in the conventional design is perturbed due to parasitic reflections.

## 2 Design of the unit-cell using 2D evanescent fields

In this work we have presented a non-local design for emulating the ideal "active-passive" behaviour. In this sense, the response is obtained not by local contribution of each array element but as a collective action of the unit cell as a whole. As a particular realization we propose an array of metallic patches with negligible electrical thickness placed above a ground plane, at a distance $t_\mathrm{d}$. In this work, the ideal performance has been obtained by using a numerical optimization. Final results of the optimization process are shown in Figs. 3(b) and 3(d). In this section we analyze these results in detail and elucidate the role of evanescent fields excited near the metasurface.

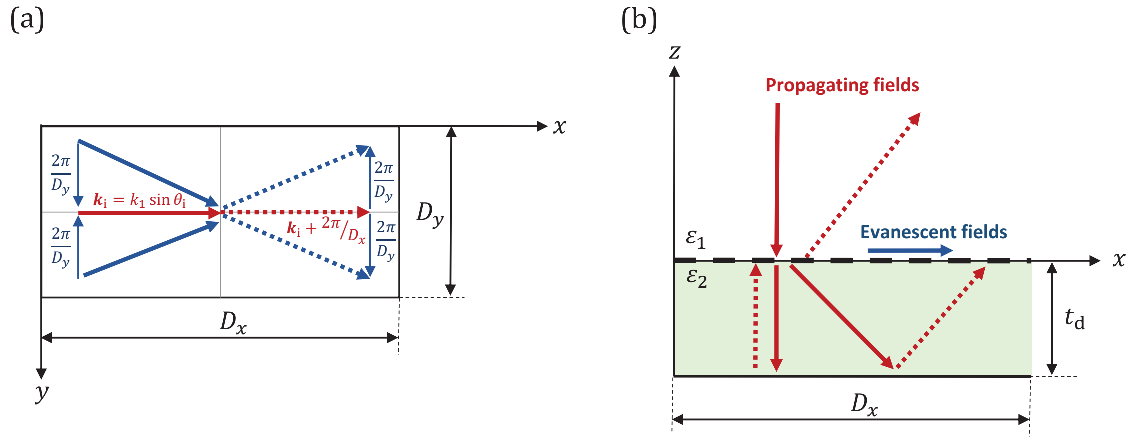


Figure 2: Illustration of the desired performance of an ideally reflecting metasurface. TE incidence is assumed and the metasurface is located in the $xy$-plane.

Because the metal patches are negligibly thin, they support only tangential electric currents. Thus, we can assume that the tangential components of the electric field are continuous across the plane of the patches. The tangential component of the electric fields in the background medium (denoted by 'b') and in the substrate (denoted by 's') can be expressed as a superposition of propagating and evanescent fields:

$$E_t^{\mathrm{b,s}} = E_{\mathrm{pr}}^{\mathrm{b,s}} + E_{\mathrm{ev}}^{\mathrm{b,s}}. \tag{8}$$

Propagating fields in the background are the superposition of the incident plane wave with the amplitude $E_{\mathrm{i}}$ and the anomalously reflected plane wave with the amplitude $E_{\mathrm{r}} = E_{\mathrm{i}}\sqrt{\frac{\cos\theta_{\mathrm{i}}}{\cos\theta_{\mathrm{r}}}}$:

$$E_{\mathrm{pr}}^{\mathrm{b}} = E_{\mathrm{i}} e^{-jk_1 \sin\theta_{\mathrm{i}} x} e^{jk_1 \cos\theta_{\mathrm{i}} z} + E_{\mathrm{r}} e^{-jk_1 \sin\theta_{\mathrm{r}} x} e^{-jk_1 \cos\theta_{\mathrm{r}} z}. \tag{9}$$

In the substrate, the propagating waves are defined by

$$E_{\mathrm{pr}}^{\mathrm{s}} = A_1 e^{-jk_1 \sin\theta_{\mathrm{i}} x}(e^{jk_{z1}z} + R_1 e^{-jk_{z1}z}) + A_2 e^{-jk_1 \sin\theta_{\mathrm{r}} x}(e^{jk_{z2}z} + R_2 e^{-jk_{z2}z}), \tag{10}$$

where $k_{z1} = k_1\sqrt{\varepsilon_2 - \sin\theta_{\mathrm{i}}^2}$ and $k_{z2} = k_1\sqrt{\varepsilon_2 - \sin\theta_{\mathrm{r}}^2}$ are the vertical wavenumbers of the propagating waves, $R_1 = -e^{-2jk_{z1}t_{\mathrm{d}}}$ and $R_2 = -e^{-2jk_{z2}t_{\mathrm{d}}}$ are the reflection coefficients from the ground plane and $t_{\mathrm{d}}$ is the thickness of the dielectric substrate. Notice that we have considered propagating waves with the same tangential wavenumbers than the ones above the metasurface.

The actual implementation of the proposed metasurface is a 2D array. All evanescent waves produced by the 2D grating should be considered, but not only the evanescent waves

related with the periodic gradient in the $x$-direction. The patches are aligned with the center at $y = 0$. Since the tangential electric field in between the patches is small, we can assume that along this symmetrically positioned line $y = 0$, $z = 0$ the tangential electric field is zero [see Fig. 3(d)]. In order to satisfy this condition, we consider evanescent fields with the same wavenumber in the $x$-direction as the propagating waves but with an addition wavenumber along the $y$-direction [see Fig. 1(a)]. The tangential component of the evanescent fields in the background is expressed as

$$E_{\rm ev}^{\rm b} = B_1 e^{-jk_1 \sin\theta_{\rm i} x} e^{-\alpha_1 z} \cos\left(\frac{2\pi}{D_{\rm y}} y\right) + B_2 e^{-jk_1 \sin\theta_{\rm r} x} e^{-\alpha_2 z} \cos\left(\frac{2\pi}{D_{\rm y}} y\right), \tag{11}$$

where $\alpha_1 = \sqrt{k_1^2 \sin\theta_{\rm i}^{\,2} + \left(\frac{2\pi}{D_{\rm y}}\right)^2 - k_1^2}$ and $\alpha_2 = \sqrt{k_1^2 \sin\theta_{\rm r}^{\,2} + \left(\frac{2\pi}{D_{\rm y}}\right)^2 - k_1^2}$ are the attenuation constants of the evanescent field. Evanescent fields in the substrate must have the same tangential wave vector as the evanescent field above the interface:

$$E_{\rm ev}^{\rm s} = B_3 e^{-jk_1 \sin\theta_{\rm i} x} (e^{\alpha_3 z} + R_3 e^{-\alpha_3 z}) \cos\left(\frac{2\pi}{D_{\rm y}} y\right) + B_4 e^{-jk_1 \sin\theta_{\rm r} x} (e^{\alpha_4 z} + R_4 e^{-\alpha_4 z}) \cos\left(\frac{2\pi}{D_{\rm y}} y\right), \tag{12}$$

where $\alpha_3 = \sqrt{k_1^2 \sin\theta_{\rm i}^{\,2} + \left(\frac{2\pi}{D_{\rm y}}\right)^2 - k_1^2 \varepsilon_2}$ and $\alpha_4 = \sqrt{k_1^2 \sin\theta_{\rm r}^{\,2} + \left(\frac{2\pi}{D_{\rm y}}\right)^2 - k_1^2 \varepsilon_2}$ are the attenuation constants of the evanescent fields in the substrate, and $R_3 = -e^{-2\alpha_3 t_{\rm d}}$ and $R_4 = -e^{-2\alpha_4 t_{\rm d}}$ are the reflection coefficients of the evanescent fields from the ground plane.

Imposing the countinuity of the tangential fields at $z = 0$ we can find the amplitudes of the waves

$$A_1 = \frac{E_{\rm i}}{1 + R_1}, \qquad A_2 = \frac{E_{\rm r}}{1 + R_2}, \tag{13}$$

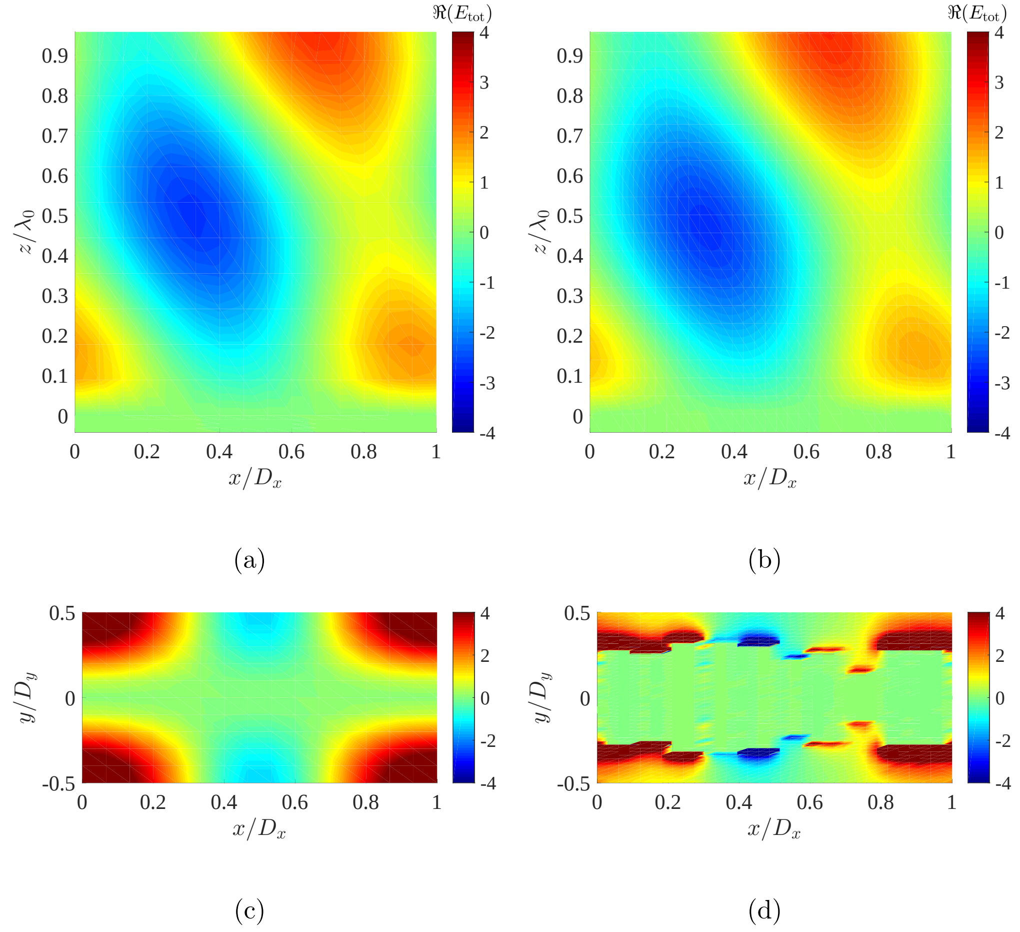


Figure 3: Real part of the total electric field. (a) and (b) represent the theoretical and simulated field distributions on the $xz$-plane when $y = 0$. (c) and (d) represent the theoretical and simulated field distributions on the $xy$-plane when $z = 0$.

$$B_3 = \frac{B_1}{1 + R_3}, \qquad B_4 = \frac{B_2}{1 + R_4}. \tag{14}$$

Now, enforcing zero tangential electric field at $y = 0$ we can find the amplitudes of the waves just defining $B_1 = -E_{\text{i}}$ and $B_2 = -E_{\text{r}}$.

Figure 3(a) shows the real part of the electric field distribution in the $xz$-plane at $y = 0$. In the bottom panel, Fig. 3(c) shows the real part of the electric field distribution

in the $xy$-plane at $z = 0$. Although this analysis is based on a number of approximations, we can see a clear concordance with the numerical optimization results, which tells that this analytical model properly describes the physical mechanism of perfect anomalous reflection.

Finally, it is important to note that at $y = \pm D_y/4$ the effect of the evanescent fields vanishes and the input impedance is the same which describes the "active-passive" behavior [Eq. (3) in the main text]. This property supports our decision to use the phase gradient defined by the "active-passive" impedance for calculating the length of each patch in the initial estimation.

## 3 Scattered fields from a reference metal plate illuminated obliquely

In this paragraph we analytically estimate scattering properties of a reference metal plate illuminated by an incident wave at an angle $\phi$. In particular, we are interested in the amplitude of the scattered wave in the specular direction, i.e. when the angles of incidence and reflection are equal. Geometry of the problem is shown in Fig. 4. The receiving antenna is located at a distance $R = 2.387$ m from the center of the plate. In addition to the Cartesian coordinate system $xyz$ used in the main text, it is convenient to introduce a local coordinate system $uyn$, where the coordinates $u$ and $y$ define the plate plane, and the axis $n$ defines its normal (for clarity not shown in the figure). We define the dimensions of the plate along $u$ and $y$ axis as $a = 440$ mm and $b = 262.5$ mm, respectively.

Assuming that the incident wave from the transmitting antenna located at $147\lambda$ dis-

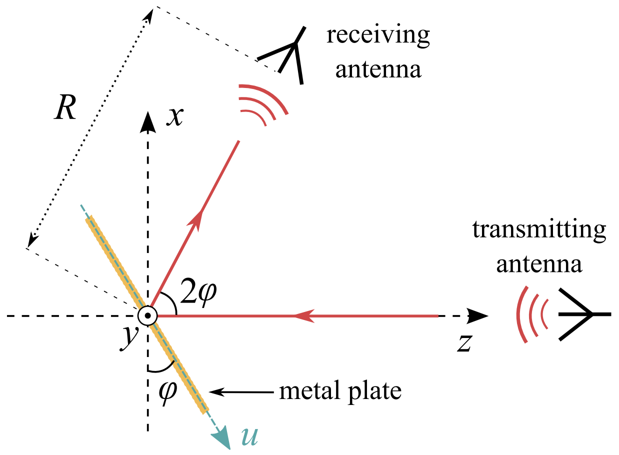


Figure 4: Geometry of the problem with a metal plate.

tance from the plate is planar, the electric current induced on the plate surface reads, in the physical optics approximation,

$$\mathbf{j}_{\mathrm{e}}(u) = \hat{y} E_0 \frac{2}{\eta_1} \cos\phi \cdot e^{jk_1 u \sin\phi}, \tag{15}$$

where $E_0$ is the incident electric field at the center of the plate, $\eta_1$ is the vacuum impedance, and $k_1$ is the wavenumber in free space. After some calculations, the distance between a current element with the coordinates $(u, y)$ and the receiving antenna can be written as

$$r(u, y) = \sqrt{u^2 + y^2 + 2uR\sin\phi + R^2}. \tag{16}$$

Next, we calculate the electric vector potential $\mathbf{A}$ created by the currents given by (15):

$$\mathbf{A} = \frac{1}{4\pi} \int\limits_S \mathbf{j}_{\mathrm{e}}(u) \frac{e^{-jk_1 r(u,y)}}{r(u,y)} \,\mathrm{d}S = \hat{y}\, \frac{E_0 \cos\phi}{2\pi\eta_1} \int_{-a/2}^{a/2} \mathrm{d}u \int_{-b/2}^{b/2} \frac{e^{jk_1[u\sin\phi - r(u,y)]}}{r(u,y)} \,\mathrm{d}y, \tag{17}$$

where $\mathrm{d}S = \mathrm{d}u\mathrm{d}y$ is the area element of the metal plate. The scattered electric field from

the plate at the location of the receiving antenna reads

$$\mathbf{E}_{\rm sc\,p} = -j\omega\mu_0\mathbf{A} = -\hat{y}\,\frac{jk_1E_0\cos\phi}{2\pi}\int_{-a/2}^{a/2}{\rm d}u\int_{-b/2}^{b/2}\frac{e^{jk_1[u\sin\phi-r(u,y)]}}{r(u,y)}\,{\rm d}y. \tag{18}$$

## 4 Scattered fields from the normally illuminated metasurface

In this paragraph we analytically estimate the scattering properties of the anomalously reflecting metasurface normally illuminated by an incident plane wave. In particular, we are interested in the amplitude of the scattered wave at an angle 70° from the normal. Geometry of the problem is shown in Fig. 5. The receiving antenna is located at the

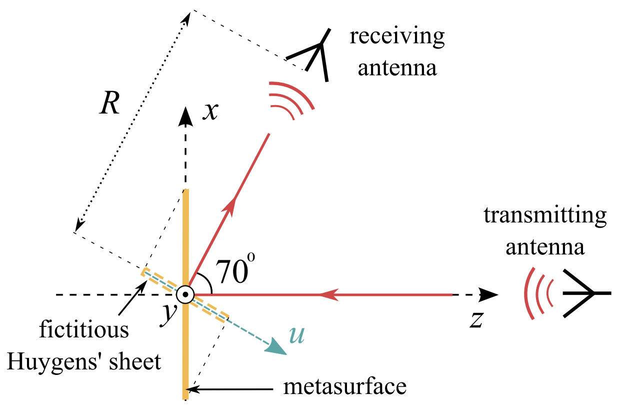


Figure 5: Geometry of the problem with a metasurface.

same distance $R = 2.387$ m from the center of the plate. In our analysis we use the idea that an ideal reflecting metasurface has the same scattering properties as a fictitious sheet of Huygens' currents (electric and magnetic) oriented orthogonally to the main reflected beam (see Fig. 5). As is seen from the illustration, the dimensions of such a fictitious current sheet are $a\cos 70°$ and $b$ along the $u$ and $y$ axes, respectively. Thus, the area of

the current sheet is smaller than that of the metasurface. This results in weaker scattering from the metasurface as compared with the reference metal plate of the same size.

To find the fictitious currents emulating the metasurface scattering, we need to know the reflected fields from the metasurface (under the assumption that the metasurface is infinite). As it was shown in the main text in Section IIC, these fields in our configuration read

$$\mathbf{E}_{\rm r} = \hat{y}\,\frac{E_0}{\sqrt{\cos 70^\circ}}, \qquad \mathbf{H}_{\rm r} = \hat{u}\,\frac{E_0}{\eta_1\sqrt{\cos 70^\circ}}. \tag{19}$$

Next, we write the fictitious Huygens' currents which emulate the same reflected fields:

$$\mathbf{j}_{\rm e} = -\hat{y}\,\frac{E_0}{\eta_1\sqrt{\cos 70^\circ}}, \qquad \mathbf{j}_{\rm m} = -\hat{u}\,\frac{E_0}{\sqrt{\cos 70^\circ}}. \tag{20}$$

Note that these currents are uniform and do not depend on the coordinates at the sheet. Next, we calculate the scattered fields from the electric currents. It can be shown that the scattered fields from the magnetic currents are identical. As is seen from Fig. 5, the distance between a current element with the coordinates $(u, y)$ and the receiving antenna can be written as

$$r(u,y) = \sqrt{u^2 + y^2 + R^2}. \tag{21}$$

Next, we calculate the electric vector potential $\mathbf{A}$ created by the electric currents:

$$\mathbf{A} = \frac{1}{4\pi}\int\limits_S \mathbf{j}_{\rm e}\frac{e^{-jk_1 r(u,y)}}{r(u,y)}\,{\rm d}S = -\hat{y}\,\frac{E_0}{4\pi\eta_1\cos 70^\circ}\int_{-a/2\cos 70^\circ}^{a/2\cos 70^\circ}{\rm d}u\int_{-b/2}^{b/2}\frac{e^{-jk_1 r(u,y)}}{r(u,y)}\,{\rm d}y. \tag{22}$$

The scattered electric field from the metasurface at the location of the receiving antenna will be double of the field scattered by the electric currents at the sheet (the electric and

magnetic currents have equal contributions):

$$\mathbf{E}_{\mathrm{sc\,m}} = \hat{y}\,\frac{jk_1E_0}{2\pi\cos 70^\circ}\int_{-a/2\cos 70^\circ}^{a/2\cos 70^\circ}\mathrm{d}u\int_{-b/2}^{b/2}\frac{e^{-jk_1r(u,y)}}{r(u,y)}\,\mathrm{d}y. \tag{23}$$

## 5 Correction factor for the signal amplitudes measured in the experiment

The correction factor introduced in the main text represents the ratio between the theoretically calculated signal amplitudes from the ideal metasurface and a reference perfect conductor plate $\xi_0 = |S_{21,0\mathrm{m}}|/|S_{21,0\mathrm{p}}|$. Obviously, this ratio is equal to the ratio between the amplitude of the scattered electric fields in the two cases, i.e. $\xi_0 = |E_{\mathrm{sc\,m}}/E_{\mathrm{sc\,p}}|$. Using expressions (18) and (23) and assuming $\phi = 35^\circ$, we find that for our configuration $\xi_0 = 0.758 = -2.41$ dB. Interestingly, when the distance between the receiving antenna and the metasurface $R$ tends to infinity, the correction factor can be calculated using a simple trigonometric formula: $\xi_0 = \sqrt{\cos 70^\circ}/\cos\phi$.
